# Supplementary material for: End-User Programming of Low- and High-Level Actions for Robotic Task Planning
Source: arXiv:2103.14342 source file (2021-03-26)
Supplement: Supplementary file 1 [file appendix.tex]

\appendix
\label{sec:appendix}
PDDL code generated by users at the end of the user study using our graphical interface.
\begin{verbatim}
(define (domain BAXTER)
 (:requirements :typing :strips)
 (:types 
    object - element
    position - element
    cube - object
    roof - object
    base - object)
 (:predicates
    (clear ?e - element)
    (on ?o - object ?l - element)
    (stackable-on ?o - object ?l - element))
 (:action move-grip
   :parameters  (?obj - roof ?from - element 
                 ?to - element)
   :precondition (and (on ?obj ?from) 
                      (clear ?from)
                      (is-stackable ?obj ?to))
   :effect (and (on ?obj ?to) (clear ?to)
                not(on ?obj ?from) not(clear ?to))
 (:action move-suction
   :parameters  (?obj - object ?from - element 
                 ?to - element)
   :precondition (and (on ?obj ?from) 
                      (clear ?from)
                      (clear ?obj) (is-flat ?obj)
                      (is-stackable ?obj ?to))
   :effect (and (on ?obj ?to) (clear ?to)
                not(on ?obj ?from) not(clear ?to))
 )
 
 (define (problem build-house)
    (:domain BAXTER)
  (:objects
    a b c - cube
    t1 t2 t3 - position)
  (:init (and (on a t1) (on b a) (clear b) 
              (clear t2) (clear t3)))
  (:goal (and (on a b) (on b t3)))
)
\end{verbatim}
